# Supplementary material for: A Robust Seemingly Unrelated Regressions For Row-Wise And Cell-Wise Contamination
Source: arXiv:2107.00975 source file (2021-07-02)
Supplement: Supplementary file 1 [file supplemental.pdf]

# Supplemental Material for "A Robust Seemingly Unrelated Regressions For Row-Wise And Cell-Wise Contaminations"

Giovanni Saraceno[1], Fatemah Alqallaf[2], and Claudio Agostinelli[1]

[1]*Department of Mathematics, University of Trento, Trento, Italy*
[2]*Department of Statistics and Operational Research, Kuwait University, Kuwait*

July 2, 2021

## Introduction

In Section SM–1 of this supplemental material we describe the R package `robustsur` while in Section SM–2 we report the complete results of the Monte Carlo simulation described in Section 4.

## SM–1 Illustration of the R package `robustsur`

We illustrate the use of the R package `robustsur` (version 0.0.6) using the data set `Kmenta` (Kmenta, 1986) available in the R package `systemfit` (Henningsen and Hamann, 2007).

```
> library(robustsur)
> library(systemfit)
> data(Kmenta)
```

We consider a simple setting with two equations

```
> eqDemand <- consump~price+income
> eqSupply <- consump~price+farmPrice+trend
> system <- list(demand=eqDemand, supply=eqSupply)
```

## SM–1-1 Analysis of the original dataset

From the point of view of the user, the function `surerob` is essentially used in the same way as the function `systemfit`

```
> fitols <- systemfit(system, data=Kmenta)
> fitrob <- surerob(system, data=Kmenta)
```

However, the function `surerob` has only three arguments:

`formula` : it is used to specify the form of all the equations in a `list` object;

`data` : it is used to specify the data set; in case a different data set is used for each equation, they must be specified in a `list` object;

`control` : it is used to pass control parameters to the function that performs robust estimation of the parameters for each equation, i.e. the function `lmrob` from the R package `robustbase` (Mächler et al., 2021), and it must have the same structure as the function `lmrob.control` from the same package.

`...` : it is used to pass control parameters to the function that performs robust estimation of the variance-covariance structure, i.e. the function `TSGS` from the R package `GSE` (Leung et al., 2019), see the help page of this function for the list of all available parameters.

The shape of the `print` method is the same. We notice small differences in the estimated parameters.

```
> print(fitols)

systemfit results
method: OLS

Coefficients:
demand_(Intercept)       demand_price      demand_income supply_(Intercept)
         99.895423          -0.316299           0.334636          58.275431
      supply_price  supply_farmPrice       supply_trend
          0.160367           0.248133           0.248302

> print(fitrob)
```

```
surerob results
method: Robust SUR

Coefficients:
demand_(Intercept)       demand_price      demand_income supply_(Intercept)
        103.137459          -0.412045           0.397741          53.877521
      supply_price   supply_farmPrice       supply_trend
          0.212266           0.257437           0.135818
```

Also the structure of the `summary` method is very similar. We notice small differences espcially in the p–values of the `price` variables in both equations. This is probably due to the presence of two mild outliers as shown in Figure 1.

```
> summary(fitols)

systemfit results
method: OLS

        N DF     SSR detRCov   OLS-R2 McElroy-R2
system 40 33 155.883 4.43485 0.709298   0.557559

        N DF     SSR     MSE    RMSE       R2   Adj R2
demand 20 17 63.3317 3.72539 1.93013 0.763789 0.735999
supply 20 16 92.5511 5.78444 2.40509 0.654807 0.590084

The covariance matrix of the residuals
        demand  supply
demand 3.72539 4.13696
supply 4.13696 5.78444

The correlations of the residuals
         demand   supply
demand 1.000000 0.891179
supply 0.891179 1.000000


OLS estimates for 'demand' (equation 1)
```

```
Model Formula: consump ~ price + income

              Estimate Std. Error  t value   Pr(>|t|)
(Intercept) 99.8954229  7.5193621 13.28509 2.0906e-10 ***
price       -0.3162988  0.0906774 -3.48818  0.0028153 **
income       0.3346356  0.0454218  7.36729 1.0999e-06 ***
---
Signif. codes:  0 ‘***’ 0.001 ‘**’ 0.01 ‘*’ 0.05 ‘.’ 0.1 ‘ ’ 1

Residual standard error: 1.930127 on 17 degrees of freedom
Number of observations: 20 Degrees of Freedom: 17
SSR: 63.33165 MSE: 3.725391 Root MSE: 1.930127
Multiple R-Squared: 0.763789 Adjusted R-Squared: 0.735999


OLS estimates for 'supply' (equation 2)
Model Formula: consump ~ price + farmPrice + trend

              Estimate Std. Error t value   Pr(>|t|)
(Intercept) 58.2754312 11.4629099 5.08383 0.00011056 ***
price        0.1603666  0.0948839 1.69013 0.11038810
farmPrice    0.2481333  0.0461879 5.37226 6.2274e-05 ***
trend        0.2483023  0.0975178 2.54623 0.02156713 *
---
Signif. codes:  0 ‘***’ 0.001 ‘**’ 0.01 ‘*’ 0.05 ‘.’ 0.1 ‘ ’ 1

Residual standard error: 2.405087 on 16 degrees of freedom
Number of observations: 20 Degrees of Freedom: 16
SSR: 92.551058 MSE: 5.784441 Root MSE: 2.405087
Multiple R-Squared: 0.654807 Adjusted R-Squared: 0.590084

> summary(fitrob)

robustsur results
method: Robust SUR

        N DF     SSR detRCov       R2 Adjusted R2
system 40 33 129.774 14.7777 0.706421    0.653043
```

```
        N DF      SSR       R2   Adj R2
demand 23 17  71.5625 0.725541 0.693251
supply 24 16 108.8524 0.686980 0.628289

The covariance matrix of the residuals used for estimation
        demand  supply
demand 3.01433 2.20517
supply 2.20517 2.84838

The covariance matrix of the residuals
        demand  supply
demand 3.06263 1.90855
supply 1.90855 6.01455

The correlations of the residuals
         demand   supply
demand 1.000000 0.593113
supply 0.593113 1.000000


Robust SUR estimates for 'demand' (equation 1)
Model Formula: consump ~ price + income

Call:
lmrob(formula = formula[[i]], data = data, y = TRUE, control = control)
 \--> method = "M-SMDM-M"
Residuals:
      Min         1Q    Median        3Q       Max
-4.148809 -0.888817  0.529248  1.675088  3.183846

Coefficients:
               Estimate  Std. Error  t value   Pr(>|t|)
(Intercept) 103.1374589   6.9833252 14.76910 3.9593e-11 ***
price        -0.4120448   0.0846896 -4.86535 0.00014537 ***
income        0.3977410   0.0423333  9.39546 3.8312e-08 ***
---
Signif. codes:  0 ‘***’ 0.001 ‘**’ 0.01 ‘*’ 0.05 ‘.’ 0.1 ‘ ’ 1
```

```
Robust residual standard error: 2.01275
Multiple R-squared:  0.725541,	Adjusted R-squared:  0.693251
Convergence in 9 IRWLS iterations

Robustness weights:
 one weight is ~= 1. The remaining 19 ones are summarized as
    Min.  1st Qu.   Median     Mean  3rd Qu.     Max.
0.698626 0.918369 0.953696 0.927782 0.973483 0.998695

Robust SUR estimates for 'supply' (equation 2)
Model Formula: consump ~ price + farmPrice + trend

Call:
lmrob(formula = formula[[i]], data = data, y = TRUE, control = control)
 \--> method = "M-SMDM-M"
Residuals:
      Min        1Q    Median        3Q       Max
-5.568226 -2.110513 -0.384795  0.661221  3.355917

Coefficients:
             Estimate Std. Error t value   Pr(>|t|)
(Intercept) 53.877521  12.390398 4.34833 0.00049794 ***
price        0.212266   0.101899 2.08310 0.05364202 .
farmPrice    0.257437   0.050091 5.13938 9.8909e-05 ***
trend        0.135818   0.105900 1.28251 0.21793516
---
Signif. codes:  0 ‘***’ 0.001 ‘**’ 0.01 ‘*’ 0.05 ‘.’ 0.1 ‘ ’ 1

Robust residual standard error: 1.66641
Multiple R-squared:  0.68698,	Adjusted R-squared:  0.628289
Convergence in 21 IRWLS iterations

Robustness weights:
 one weight is ~= 1. The remaining 19 ones are summarized as
    Min.  1st Qu.   Median     Mean  3rd Qu.     Max.
0.307637 0.773317 0.956860 0.853055 0.978774 0.998773
```

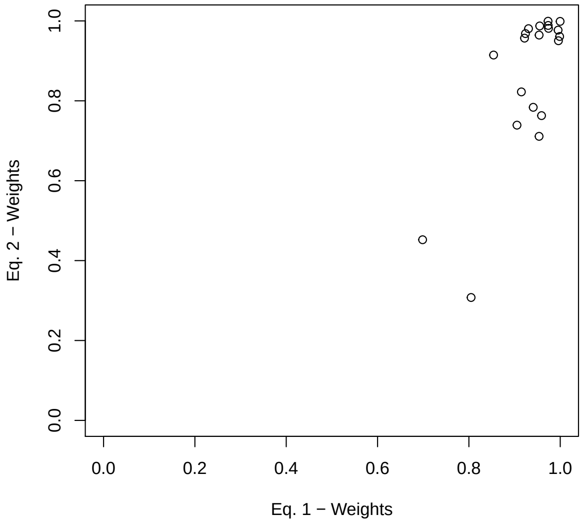


Figure 1: Original dataset. Robust weights, per equation, of each observation.

```
> plot(fitrob$rweights[,1], fitrob$rweights[,2],
+   xlim=c(0,1), ylim=c(0,1), xlab="Eq. 1 - Weights", ylab="Eq. 2 - Weights")
```

In order to see the differences in the fitted values we use the following code, which produce Figure 2 where we do not notice important differences.

```
> plot(fitrob$eq[[1]]$fitted.values, Kmenta$consump, type="n",
+   xlab="Fitted values", ylab="Food consumption",
+   main="Equation 1 - Demand", xlim=c(93,111))
> segments(x0=fitrob$eq[[1]]$fitted.values, y0=Kmenta$consump,
+   x1=fitols$eq[[1]]$fitted.values, y1=Kmenta$consump, lty=3)
> points(fitrob$eq[[1]]$fitted.values, Kmenta$consump, pch=19, col=1)
> points(fitols$eq[[1]]$fitted.values, Kmenta$consump, pch=19, col=2)
> abline(0, 1, lty=2, lwd=1.5)
> legend("bottomright", legend=c("surerob", "systemfit"),
+   col=c(1,2), pch=19, inset=0.02)
```

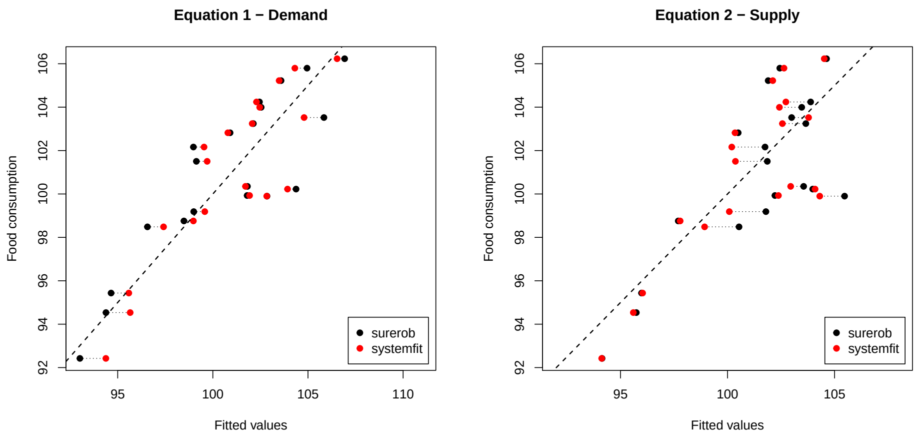


Figure 2: Original dataset. Fitted values versus dependent variable (`consump`). Black points: robust fit, red points: least square fit. The segments which connect black points to red points are used to indicate that they are related to the same observation.

```
> plot(fitrob$eq[[2]]$fitted.values, Kmenta$consump, type="n",
+   xlab="Fitted values", ylab="Food consumption",
+   main="Equation 2 - Supply", xlim=c(92,108))
> segments(x0=fitrob$eq[[2]]$fitted.values, y0=Kmenta$consump,
+   x1=fitols$eq[[2]]$fitted.values, y1=Kmenta$consump, lty=3)
> points(fitrob$eq[[2]]$fitted.values, Kmenta$consump, pch=19, col=1)
> points(fitols$eq[[2]]$fitted.values, Kmenta$consump, pch=19, col=2)
> abline(0, 1, lty=2, lwd=1.5)
> legend("bottomright", legend=c("surerob", "systemfit"),
+   col=c(1,2), pch=19, inset=0.02)
```

## SM–1-2 Analysis of a perturbed dataset

In this subsection we repeat the above analysis after an artificial perturbation of one single observations in the response variable. In particular, we modify the observation with the smallest robust weights. We arbitrarily fix it at 150.

```
> Kmenta$consump[8] <- 150
> fitols <- systemfit(system, data=Kmenta)
```

```
> fitrob <- surerob(system, data=Kmenta)

> print(fitols)

systemfit results
method: OLS

Coefficients:
demand_(Intercept)       demand_price      demand_income supply_(Intercept)
         68.893249          -0.113854           0.470575          -8.479842
      supply_price  supply_farmPrice       supply_trend
          0.615287           0.497760           0.213961

> print(fitrob)

surerob results
method: Robust SUR

Coefficients:
demand_(Intercept)       demand_price      demand_income supply_(Intercept)
         98.752697          -0.354904           0.387406          50.368013
      supply_price  supply_farmPrice       supply_trend
          0.215435           0.286350           0.175112
```

It is easy to notice important changes in the results from `systemfit` with respect to the previous, original, analysis. Indeed, all the statistically significant parameters are now not significant, $R^2$ is drastically reduced and the variance-covariance matrices and residuals sum of squares have larger order of magnitude. This is not the case for the output of `surerob`. In particular, as can be noted From Figure 3, the 8th observation is now totally discarded by the robust procedure in both equations. The changes impact also the fitted values given by the function `systemfit` as shown in Figure 4.

```
> summary(fitols)

systemfit results
method: OLS

        N DF    SSR detRCov   OLS-R2 McElroy-R2
```

```
system 40 33 3794.2 1225.73 0.256797  -0.426533

        N DF     SSR     MSE    RMSE       R2   Adj R2
demand 20 17 2035.96 119.762 10.9436 0.202400 0.108565
supply 20 16 1758.25 109.891 10.4829 0.311194 0.182043

The covariance matrix of the residuals
        demand  supply
demand 119.762 109.247
supply 109.247 109.891

The correlations of the residuals
         demand   supply
demand 1.000000 0.952294
supply 0.952294 1.000000


OLS estimates for 'demand' (equation 1)
Model Formula: consump ~ price + income

             Estimate Std. Error  t value Pr(>|t|)
(Intercept) 68.893249  42.633873  1.61593 0.124515
price       -0.113854   0.514130 -0.22145 0.827380
income       0.470575   0.257536  1.82722 0.085276 .
---
Signif. codes:  0 ‘***’ 0.001 ‘**’ 0.01 ‘*’ 0.05 ‘.’ 0.1 ‘ ’ 1

Residual standard error: 10.943588 on 17 degrees of freedom
Number of observations: 20 Degrees of Freedom: 17
SSR: 2035.955908 MSE: 119.762112 Root MSE: 10.943588
Multiple R-Squared: 0.2024 Adjusted R-Squared: 0.108565


OLS estimates for 'supply' (equation 2)
Model Formula: consump ~ price + farmPrice + trend

             Estimate Std. Error  t value Pr(>|t|)
(Intercept) -8.479842  49.962519 -0.16972 0.867355
```

```
price        0.615287   0.413563  1.48777 0.156254
farmPrice    0.497760   0.201316  2.47254 0.025017 *
trend        0.213961   0.425043  0.50339 0.621551
---
Signif. codes:  0 ‘***’ 0.001 ‘**’ 0.01 ‘*’ 0.05 ‘.’ 0.1 ‘ ’ 1

Residual standard error: 10.482869 on 16 degrees of freedom
Number of observations: 20 Degrees of Freedom: 16
SSR: 1758.248646 MSE: 109.89054 Root MSE: 10.482869
Multiple R-Squared: 0.311194 Adjusted R-Squared: 0.182043
```

*> summary(fitrob)*

```
robustsur results
method: Robust SUR

        N DF     SSR detRCov       R2 Adjusted R2
system 40 33 101.141 11.2041 0.769759    0.727897

        N DF     SSR       R2   Adj R2
demand 23 17 2234.96 0.780837 0.755053
supply 24 16 2030.17 0.758604 0.713342

The covariance matrix of the residuals used for estimation
        demand  supply
demand 2.98243 1.78902
supply 1.78902 2.32007

The covariance matrix of the residuals
        demand  supply
demand 3.32368 1.42098
supply 1.42098 3.97853

The correlations of the residuals
         demand   supply
demand 1.000000 0.987132
supply 0.987132 1.000000
```

```
Robust SUR estimates for 'demand' (equation 1)
Model Formula: consump ~ price + income

Call:
lmrob(formula = formula[[i]], data = data, y = TRUE, control = control)
 \--> method = "M-SMDM-M"
Residuals:
      Min        1Q    Median        3Q       Max
-4.303441 -1.162020  0.738819  1.509799 46.665716

Coefficients:
              Estimate Std. Error  t value   Pr(>|t|)
(Intercept) 98.7526974  7.3707685 13.39788 1.8324e-10 ***
price       -0.3549040  0.0885334 -4.00870 0.00090989 ***
income       0.3874063  0.0444316  8.71916 1.1090e-07 ***
---
Signif. codes:  0 ‘***’ 0.001 ‘**’ 0.01 ‘*’ 0.05 ‘.’ 0.1 ‘ ’ 1

Robust residual standard error: 2.01275
Multiple R-squared:  0.780837,        Adjusted R-squared:  0.755053
Convergence in 9 IRWLS iterations

Robustness weights:
 observation 8 is an outlier with |weight| = 0 ( < 0.005);
 one weight is ~= 1. The remaining 18 ones are summarized as
    Min.  1st Qu.   Median     Mean  3rd Qu.     Max.
0.666938 0.927346 0.958701 0.935328 0.974731 0.997521

Robust SUR estimates for 'supply' (equation 2)
Model Formula: consump ~ price + farmPrice + trend

Call:
lmrob(formula = formula[[i]], data = data, y = TRUE, control = control)
 \--> method = "M-SMDM-M"
Residuals:
      Min        1Q    Median        3Q       Max
-4.221290 -1.163944 -0.103274  1.299424 44.220307
```

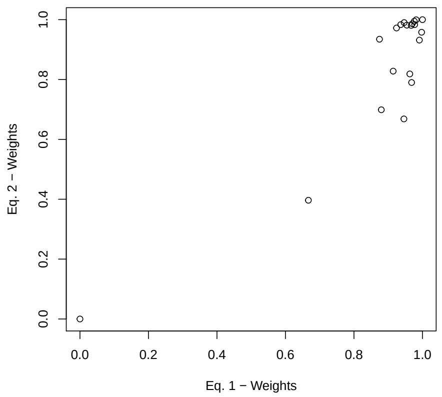


Figure 3: Perturbed dataset. Robust weights, per equation, of each observation.

```
Coefficients:
              Estimate Std. Error t value   Pr(>|t|)
(Intercept) 50.3680133 10.1960837 4.93994 0.00014775 ***
price        0.2154345  0.0834460 2.58172 0.02007168 *
farmPrice    0.2863498  0.0413025 6.93299 3.3704e-06 ***
trend        0.1751125  0.0861663 2.03226 0.05907173 .
---
Signif. codes:  0 ‘***’ 0.001 ‘**’ 0.01 ‘*’ 0.05 ‘.’ 0.1 ‘ ’ 1

Robust residual standard error: 1.66641
Multiple R-squared:  0.758604,        Adjusted R-squared:  0.713342
Convergence in 17 IRWLS iterations

Robustness weights:
 observation 8 is an outlier with |weight| = 0 ( < 0.005);
 2 weights are ~= 1. The remaining 17 ones are summarized as
    Min.  1st Qu.   Median     Mean  3rd Qu.     Max.
0.396608 0.818626 0.957892 0.876324 0.983349 0.994811
```

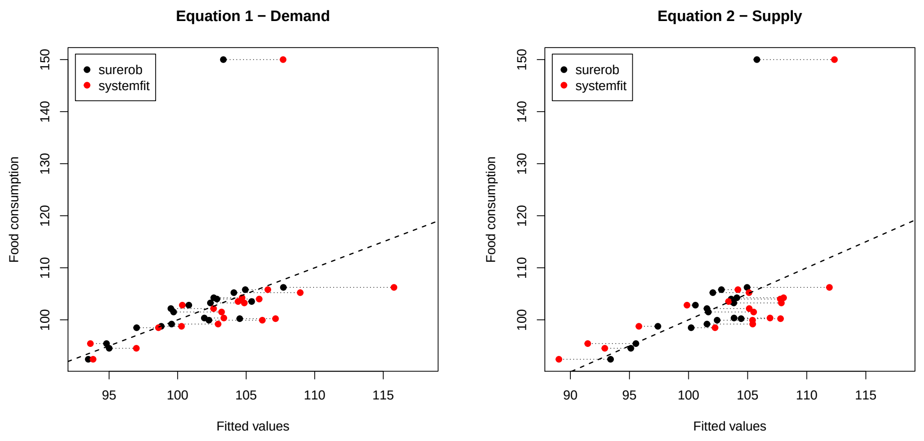


Figure 4: Perturbed dataset. Fitted values versus dependent variable (`consump`). Black points: robust fit, red points: least square fit. The segments between black points and red points are used to indicate that they are related to the same observation.

## SM–2 Complete results of the Monte Carlo Simulation

Hereafter we report the complete results of the Monte Carlo Simulation described in Section 4.

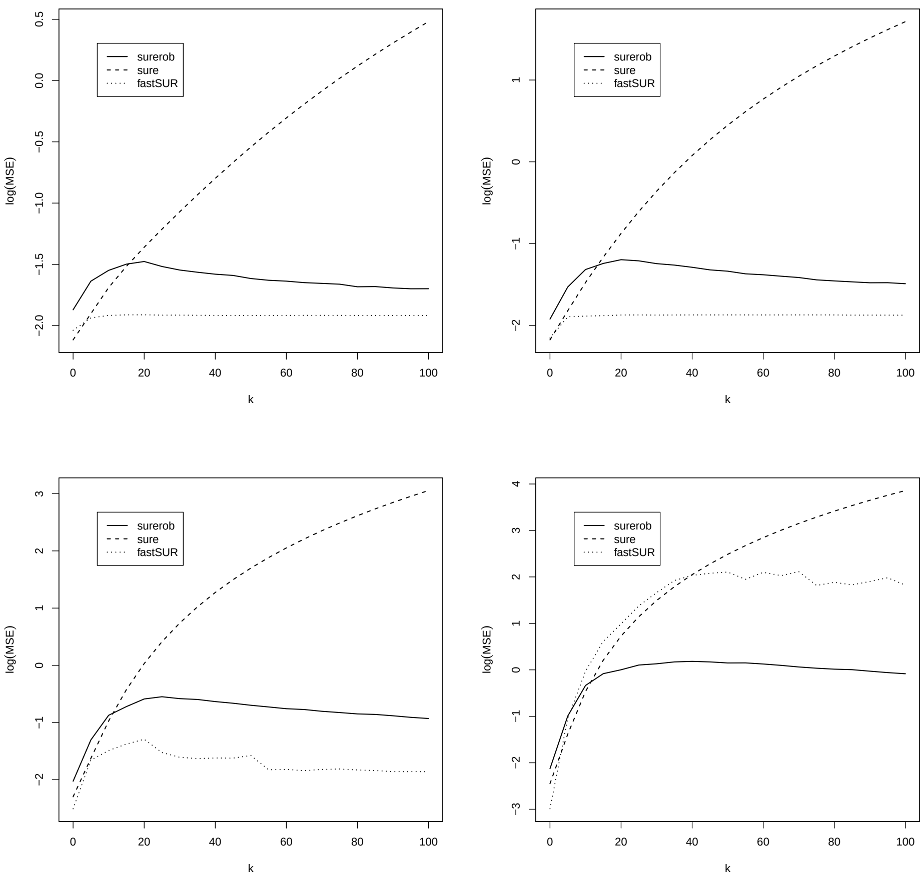


Figure 5: Mean Square Error MSE = MSE($\hat{\boldsymbol{\beta}}, \boldsymbol{\beta}$) for surerob (solid line), sure (dashed line) and FastSUR (dotted line) for different levels of contamination $\epsilon = 5\%$, $10\%$, (top) $20\%$, $30\%$ (bottom) under the THCM considering dimension $p = 5$ and number of equations $m = 5$.

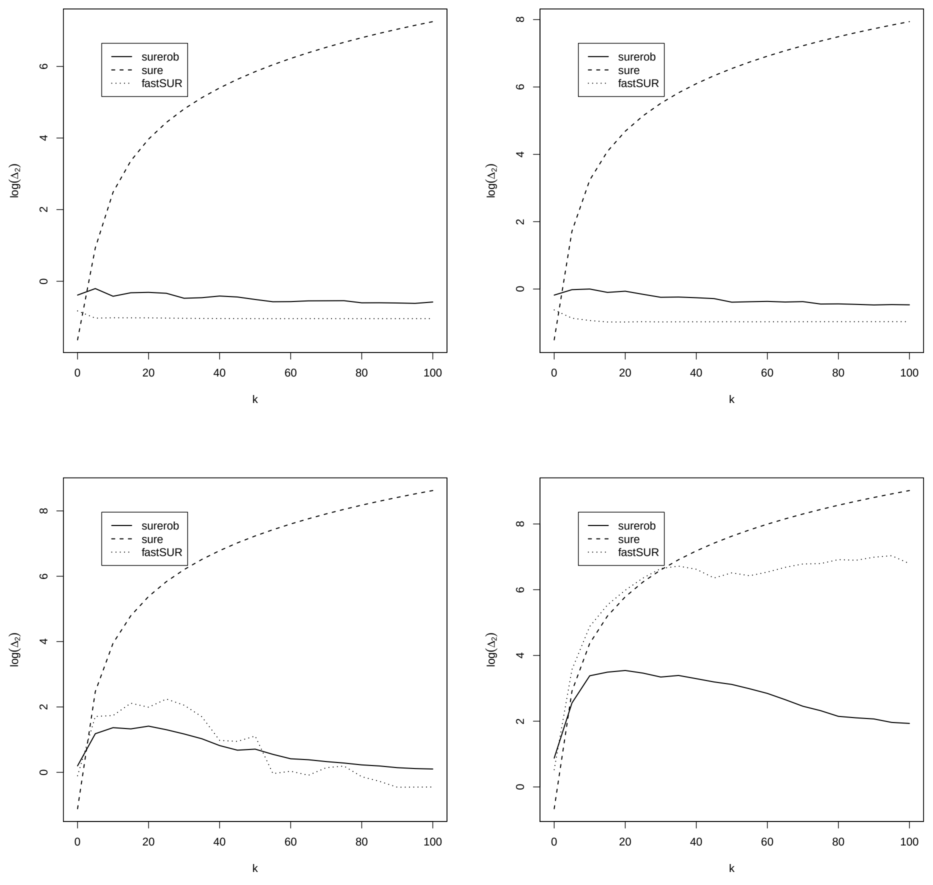


Figure 6: Average Kullback-Leibler $\Delta_2 = \Delta(\hat{\Sigma}_2, \Sigma)$ for surerob (solid line), sure (dashed line) and FastSUR (dotted line) for different levels of contamination $\epsilon = 5\%$, 10%, (top) 20%, 30% (bottom) under the THCM considering dimension $p = 5$ and number of equations $m = 5$.

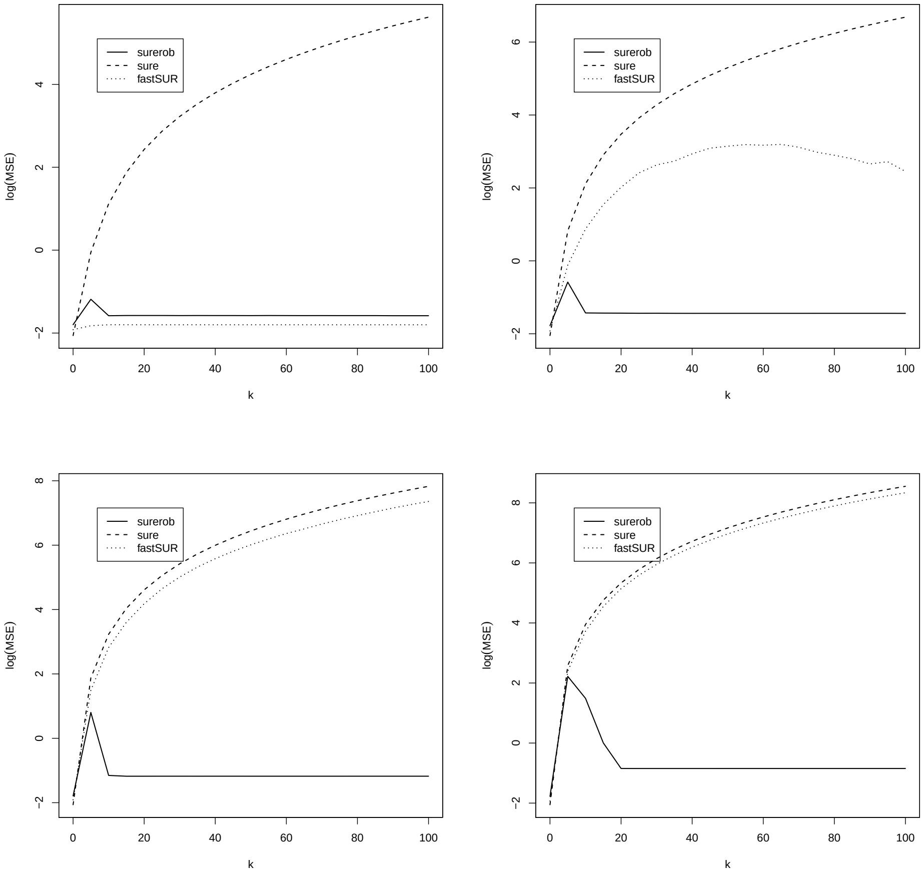


Figure 7: Mean Square Error MSE = MSE($\hat{\boldsymbol{\beta}}, \boldsymbol{\beta}$) for surerob (solid line), sure (dashed line) and FastSUR (dotted line) for different levels of contamination $\epsilon = 5\%$, 10%, (top) 20%, 30% (bottom) under the ICM considering dimension $p = 5$ and number of equations $m = 5$.

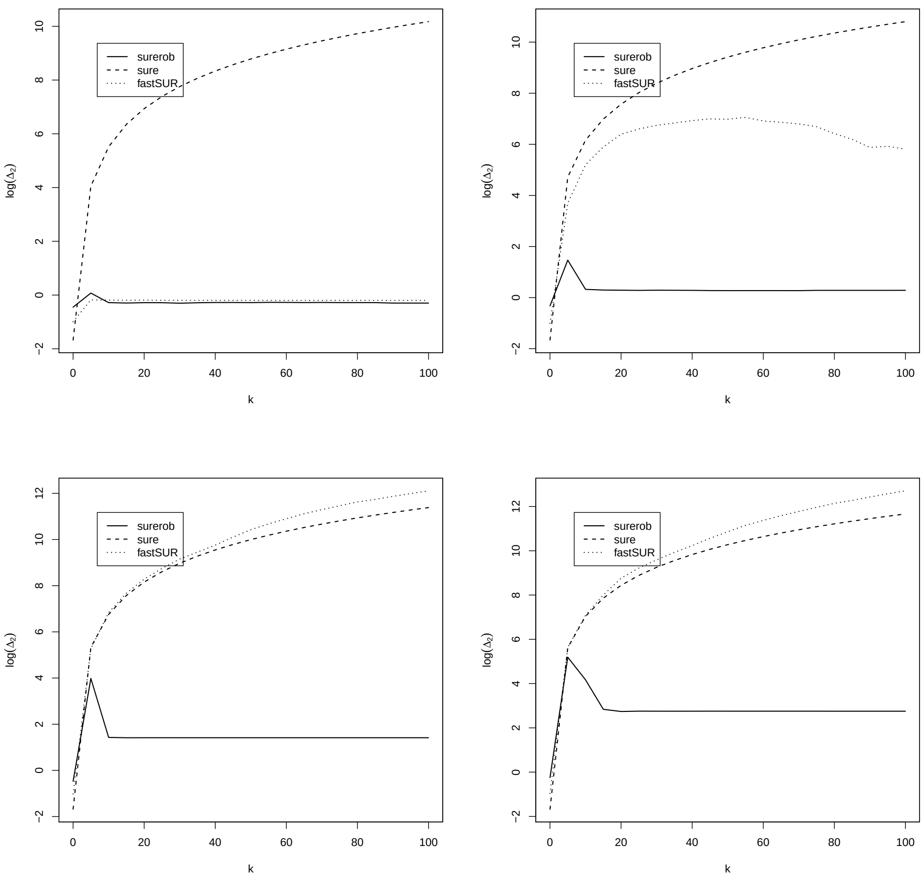


Figure 8: Average Kullback-Leibler $\Delta_2 = \Delta(\hat{\Sigma}_2, \Sigma)$ for surerob (solid line), sure (dashed line) and FastSUR (dotted line) for different levels of contamination $\epsilon = 5\%$, $10\%$, (top) $20\%$, $30\%$ (bottom) under the ICM considering $p = 5$ and number of equations $m = 5$.

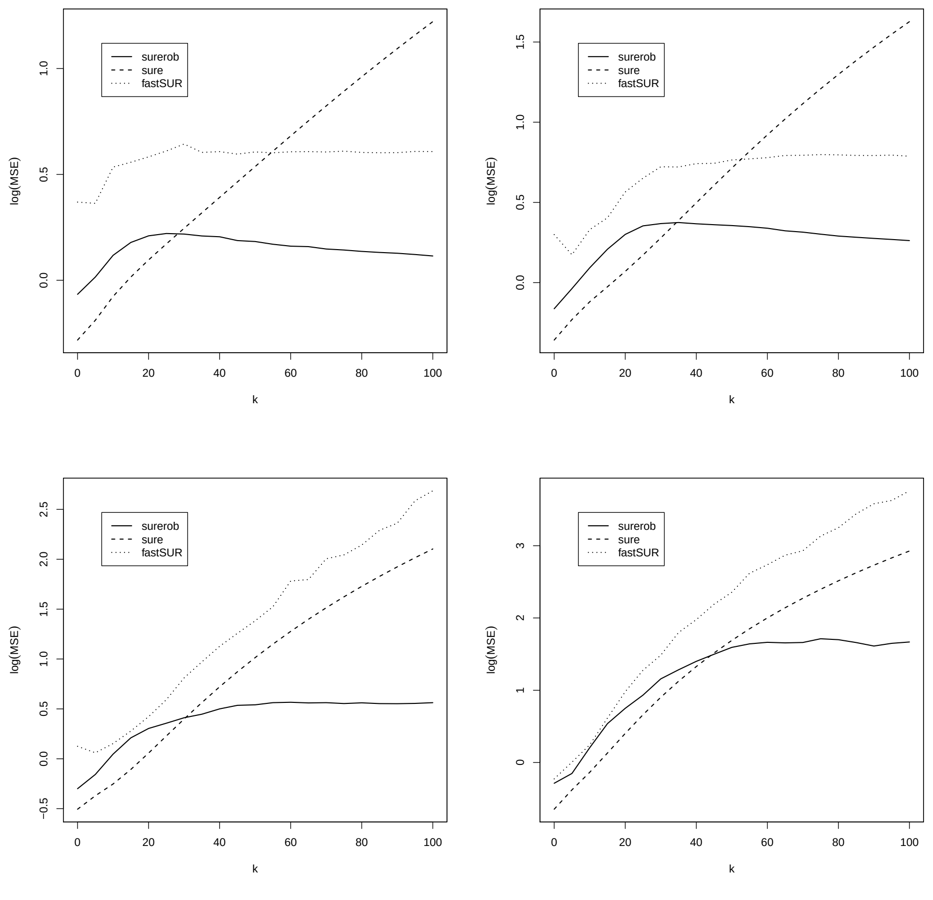


Figure 9: Mean Square Error MSE = MSE($\hat{\boldsymbol{\beta}}, \boldsymbol{\beta}$) for surerob (solid line), sure (dashed line) and FastSUR (dotted line) for different levels of contamination $\epsilon = 5\%$, $10\%$, (top) $20\%$, $30\%$ (bottom) under the THCM considering dimension $p = 5$ and number of equations $m = 20$.

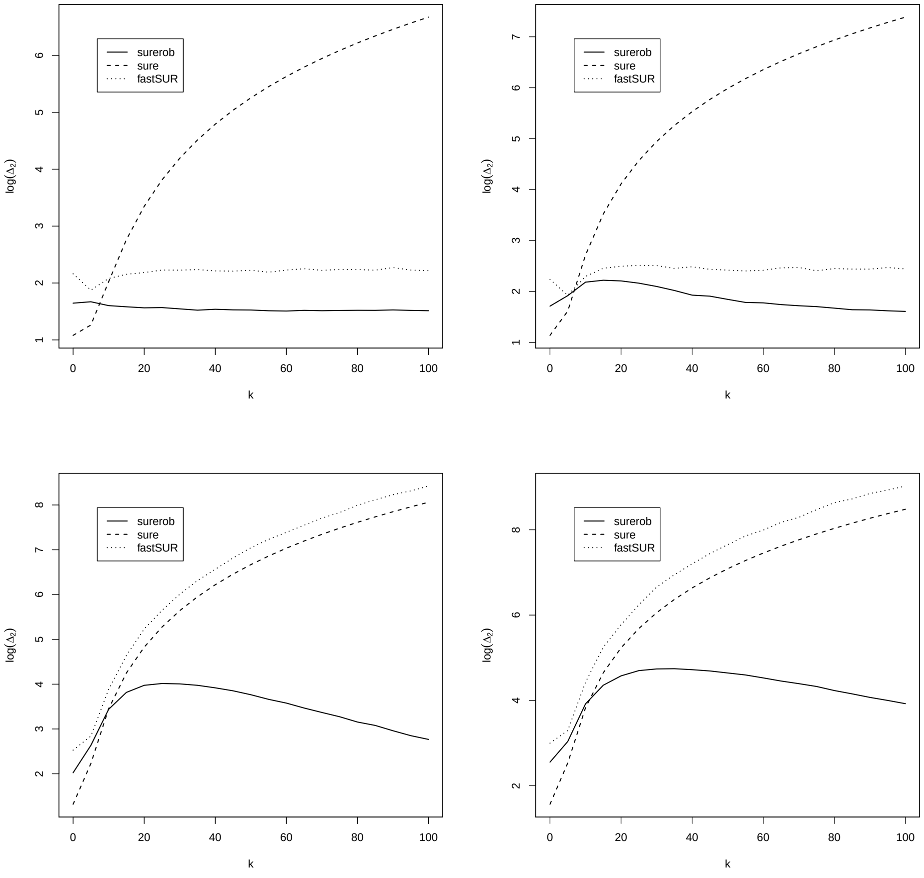


Figure 10: Average Kullback-Leibler $\Delta_2 = \Delta(\hat{\Sigma}_2, \Sigma)$ for surerob (solid line), sure (dashed line) and FastSUR (dotted line) for different levels of contamination $\epsilon = 5\%$, $10\%$, (top) $20\%$, $30\%$ (bottom) under the THCM considering dimension $p = 5$ and number of equations $m = 20$.

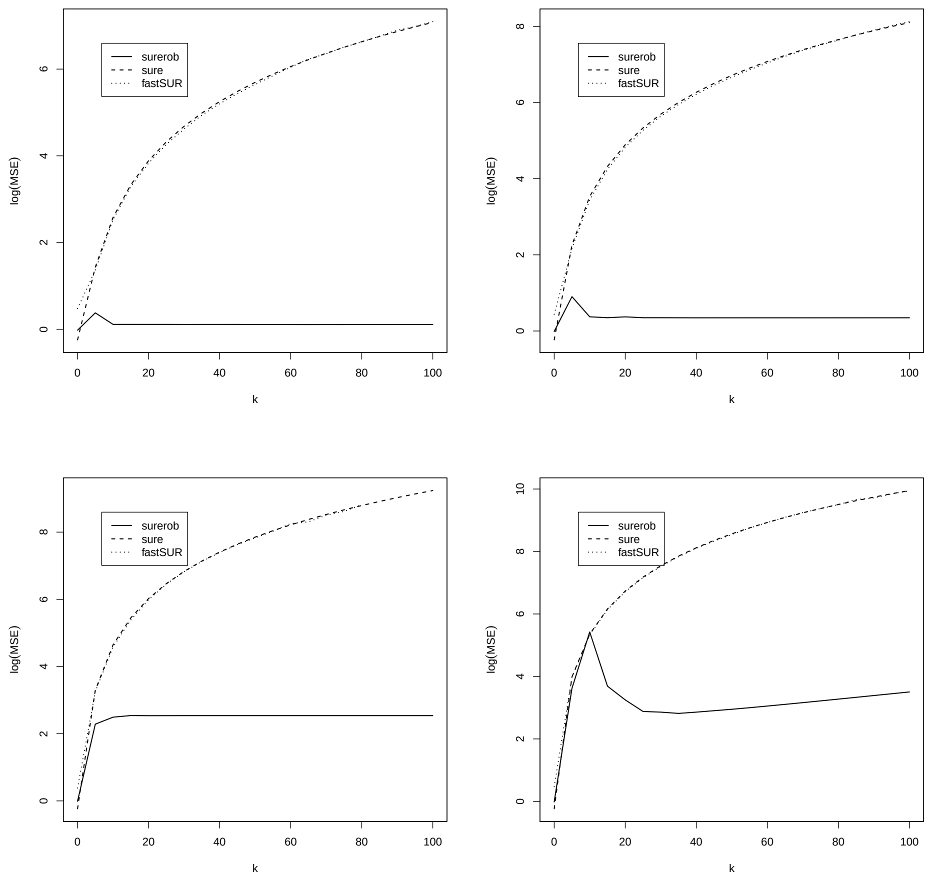


Figure 11: Mean Square Error MSE = MSE($\hat{\boldsymbol{\beta}}, \boldsymbol{\beta}$) for surerob (solid line), sure (dashed line) and FastSUR (dotted line) for different levels of contamination $\epsilon = 5\%$, $10\%$, (top) $20\%$, $30\%$ (bottom) under the ICM considering dimension $p = 5$ and number of equations $m = 20$.

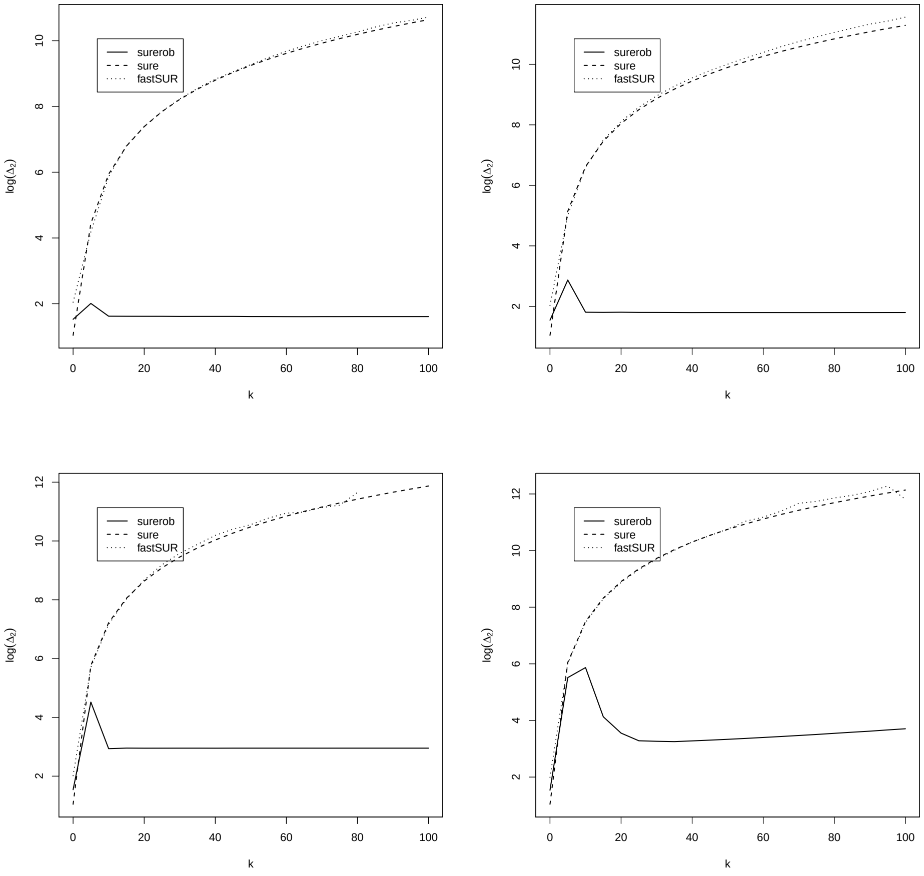


Figure 12: Average Kullback-Leibler $\Delta_2 = \Delta(\hat{\Sigma}_2, \Sigma)$ for surerob (solid line), sure (dashed line) and FastSUR (dotted line) for different levels of contamination $\epsilon = 5\%$, $10\%$, (top) $20\%$, $30\%$ (bottom) under the ICM considering $p = 5$ and number of equations $m = 20$.

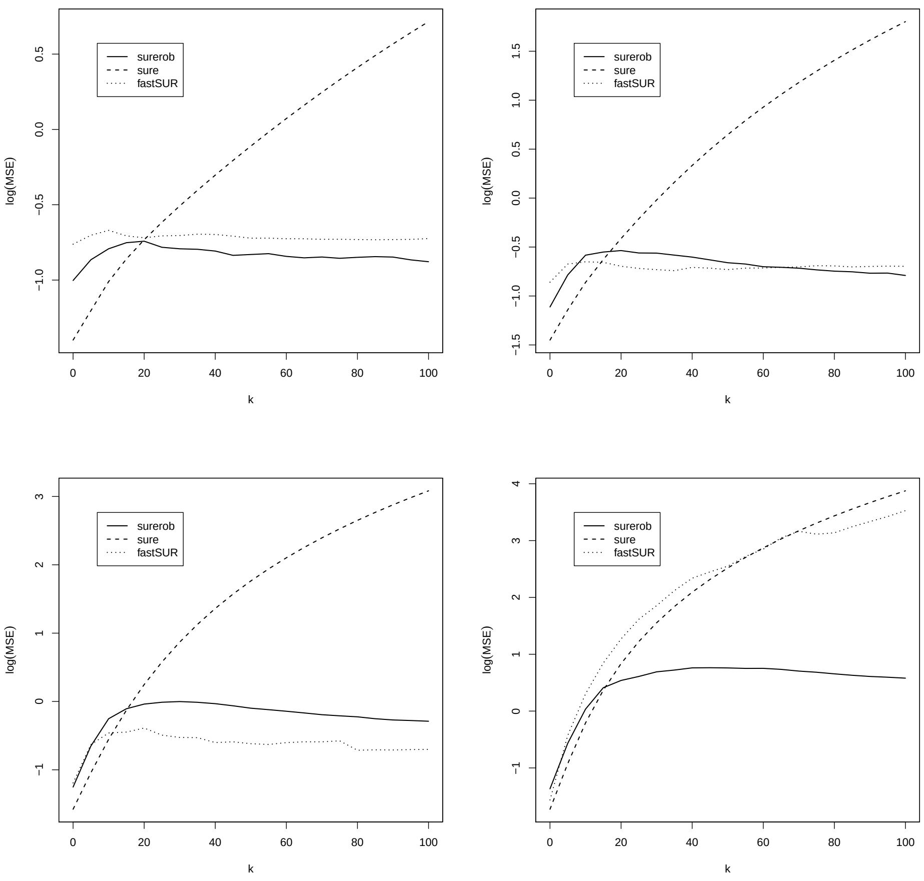


Figure 13: Mean Square Error MSE = MSE($\hat{\boldsymbol{\beta}}, \boldsymbol{\beta}$) for surerob (solid line), sure (dashed line) and FastSUR (dotted line) for different levels of contamination $\epsilon = 5\%$, $10\%$, (top) $20\%$, $30\%$ (bottom) under the THCM considering dimension $p = 10$ and number of equations $m = 5$.

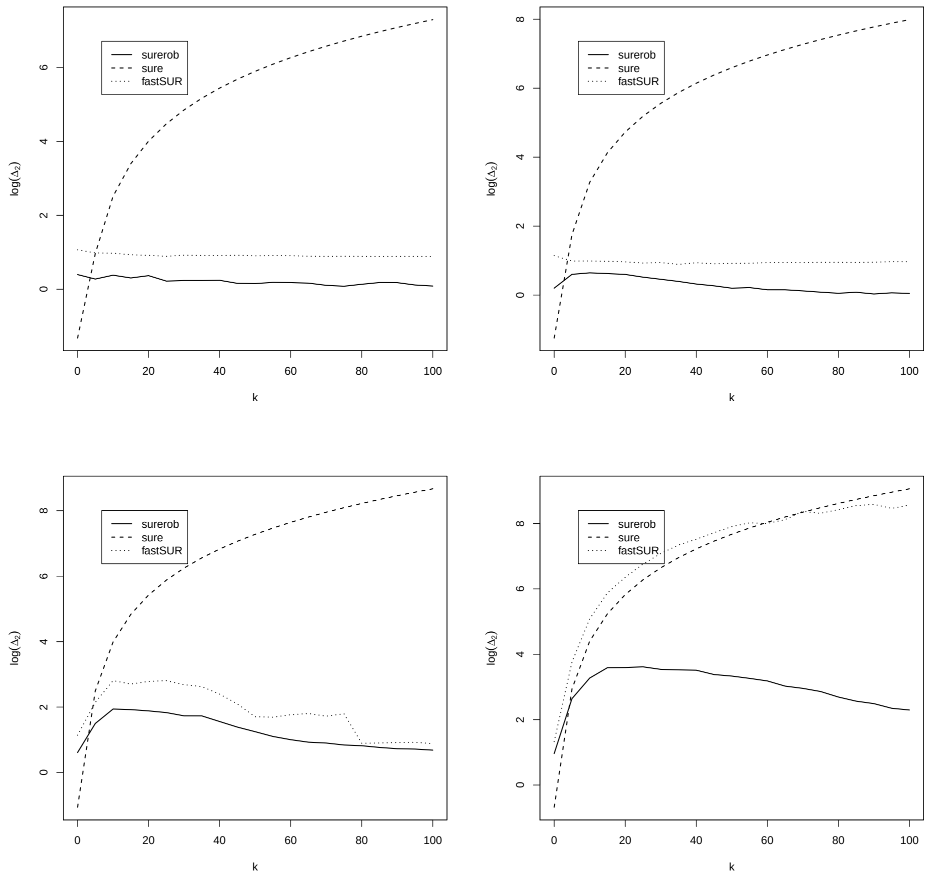


Figure 14: Average Kullback-Leibler $\Delta_2 = \Delta(\hat{\Sigma}_2, \Sigma)$ for surerob (solid line), sure (dashed line) and FastSUR (dotted line) for different levels of contamination $\epsilon = 5\%, 10\%$, (top) $20\%, 30\%$ (bottom) under the THCM considering dimension $p = 10$ and number of equations $m = 5$.

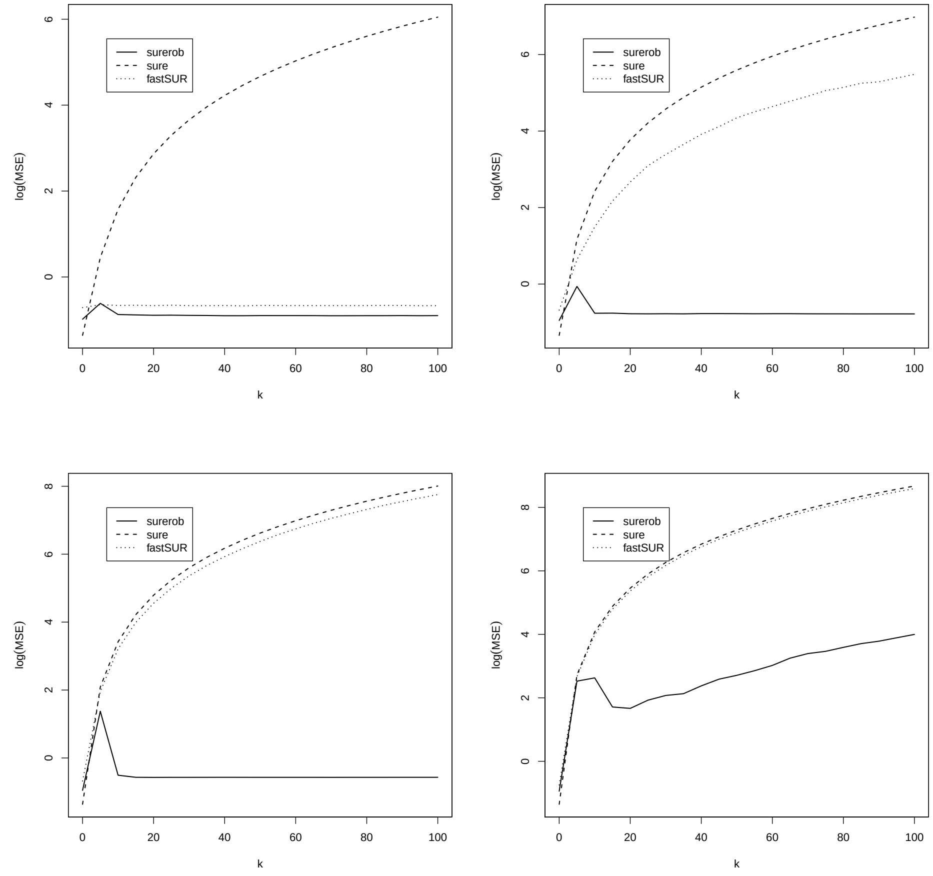


Figure 15: Mean Square Error MSE = MSE($\hat{\boldsymbol{\beta}}, \boldsymbol{\beta}$) for surerob (solid line), sure (dashed line) and FastSUR (dotted line) for different levels of contamination $\epsilon = 5\%$, $10\%$, (top) $20\%$, $30\%$ (bottom) under the ICM considering dimension $p = 10$ and number of equations $m = 5$.

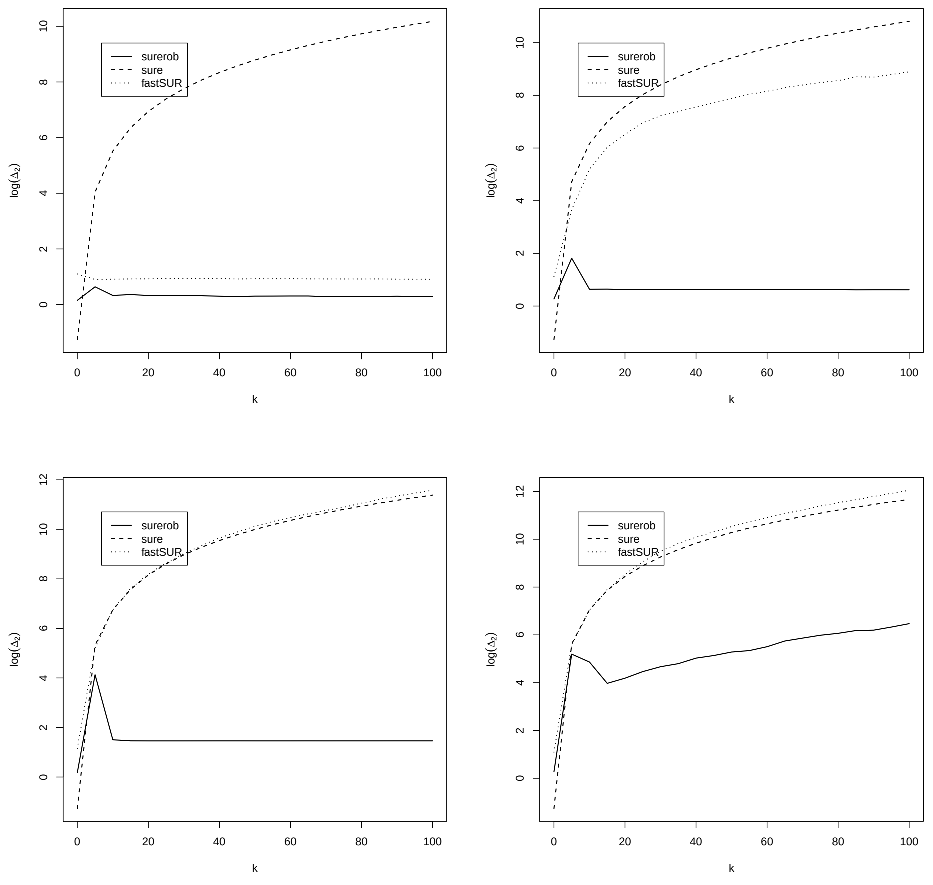


Figure 16: Average Kullback-Leibler $\Delta_2 = \Delta(\hat{\Sigma}_2, \Sigma)$ for surerob (solid line), sure (dashed line) and FastSUR (dotted line) for different levels of contamination $\epsilon = 5\%$, $10\%$, (top) $20\%$, $30\%$ (bottom) under the ICM considering $p = 10$ and number of equations $m = 5$.

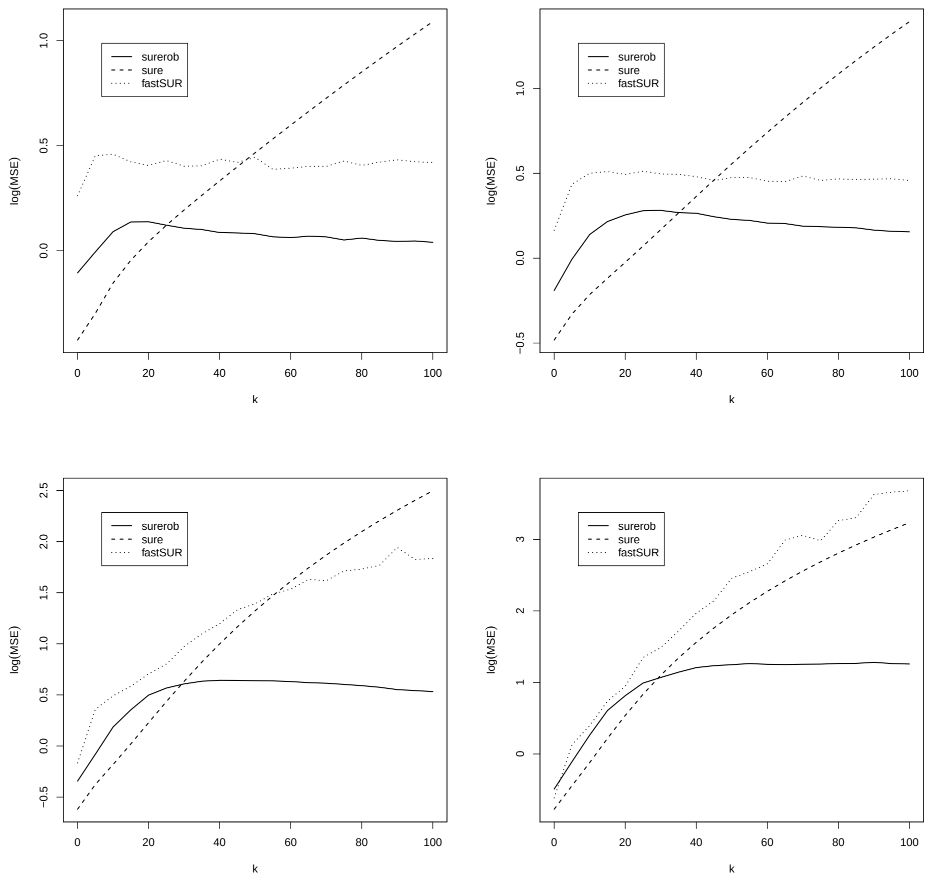


Figure 17: Mean Square Error MSE = MSE($\hat{\boldsymbol{\beta}}, \boldsymbol{\beta}$) for surerob (solid line), sure (dashed line) and FastSUR (dotted line) for different levels of contamination $\epsilon = 5\%$, 10%, (top) 20%, 30% (bottom) under the THCM considering dimension $p = 10$ and number of equations $m = 10$.

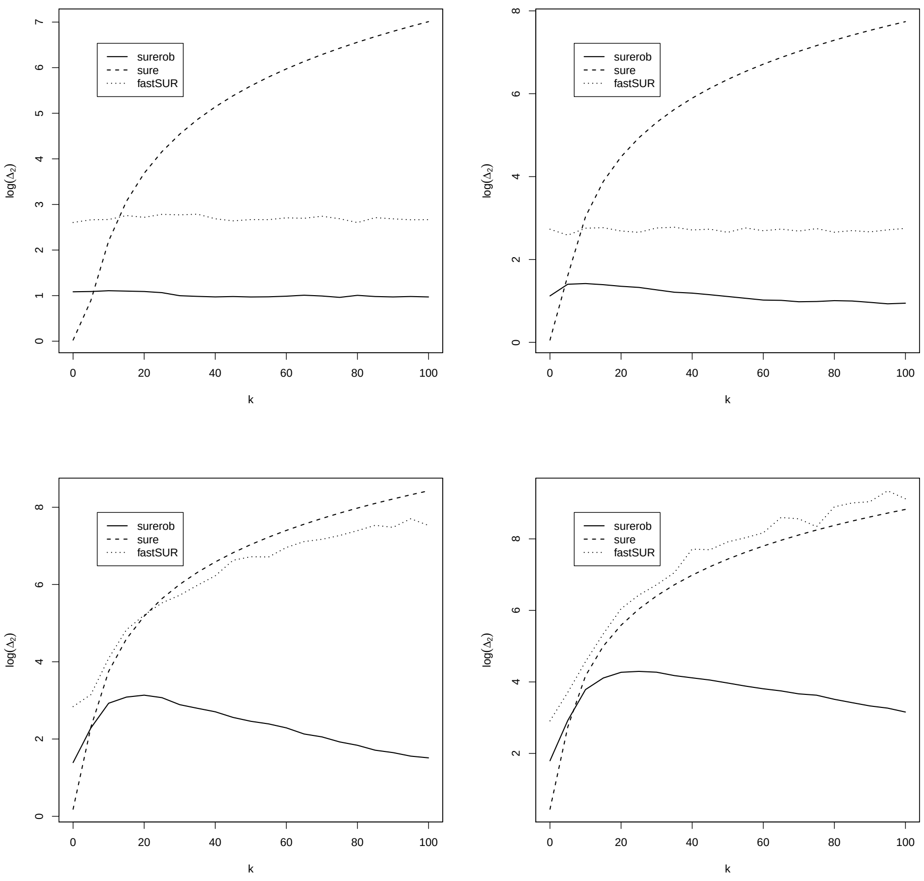


Figure 18: Average Kullback-Leibler $\Delta_2 = \Delta(\hat{\Sigma}_2, \Sigma)$ for surerob (solid line), sure (dashed line) and FastSUR (dotted line) for different levels of contamination $\epsilon = 5\%$, $10\%$, (top) $20\%$, $30\%$ (bottom) under the THCM considering dimension $p = 10$ and number of equations $m = 10$.

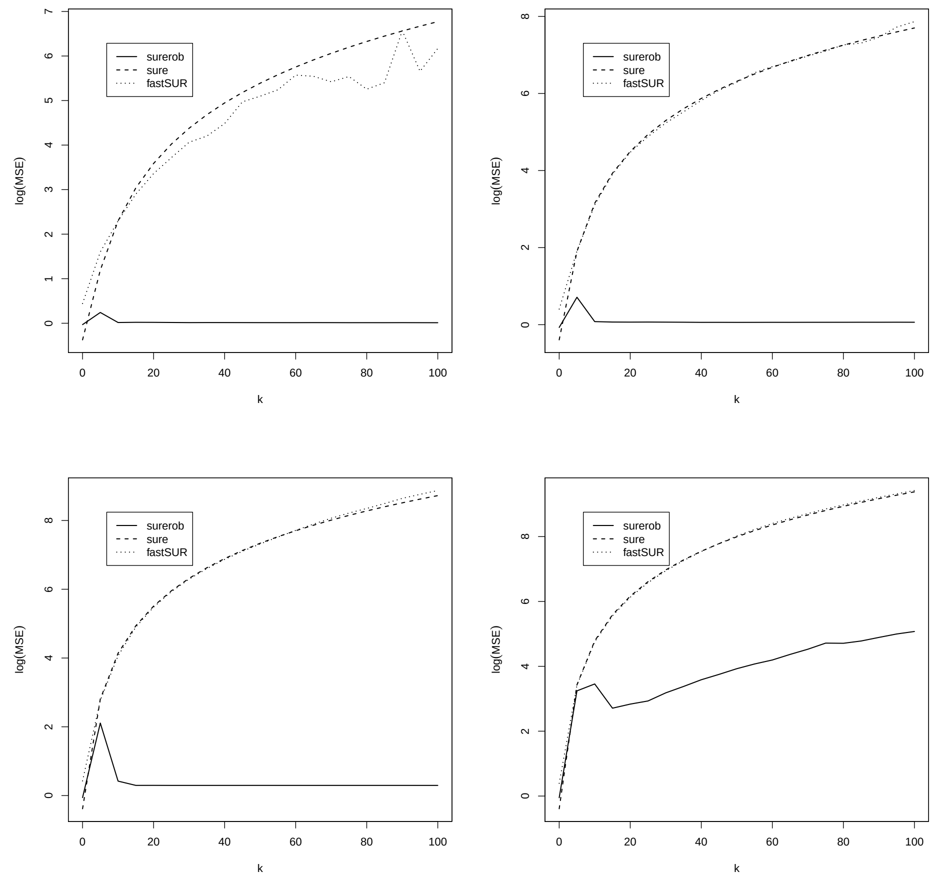


Figure 19: Mean Square Error MSE = MSE($\hat{\boldsymbol{\beta}}, \boldsymbol{\beta}$) for surerob (solid line), sure (dashed line) and FastSUR (dotted line) for different levels of contamination $\epsilon = 5\%$, $10\%$, (top) $20\%$, $30\%$ (bottom) under the ICM considering dimension $p = 10$ and number of equations $m = 10$.

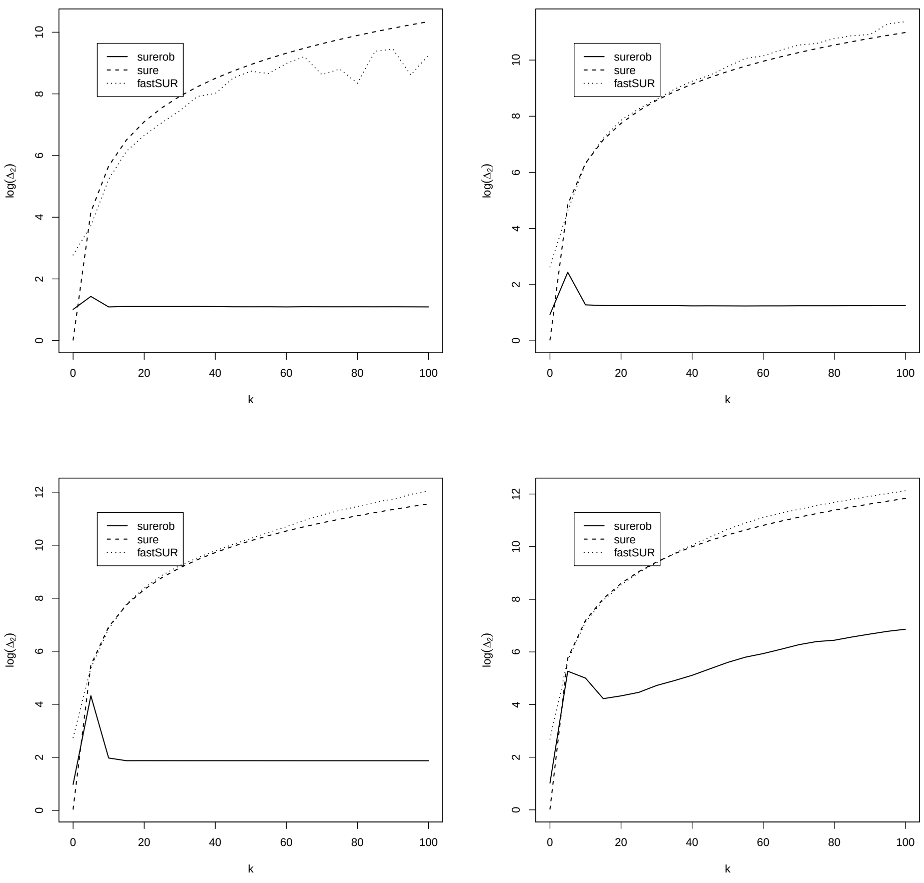


Figure 20: Average Kullback-Leibler $\Delta_2 = \Delta(\hat{\Sigma}_2, \Sigma)$ for surerob (solid line), sure (dashed line) and FastSUR (dotted line) for different levels of contamination $\epsilon = 5\%$, $10\%$, (top) $20\%$, $30\%$ (bottom) under the ICM considering $p = 10$ and number of equations $m = 10$.

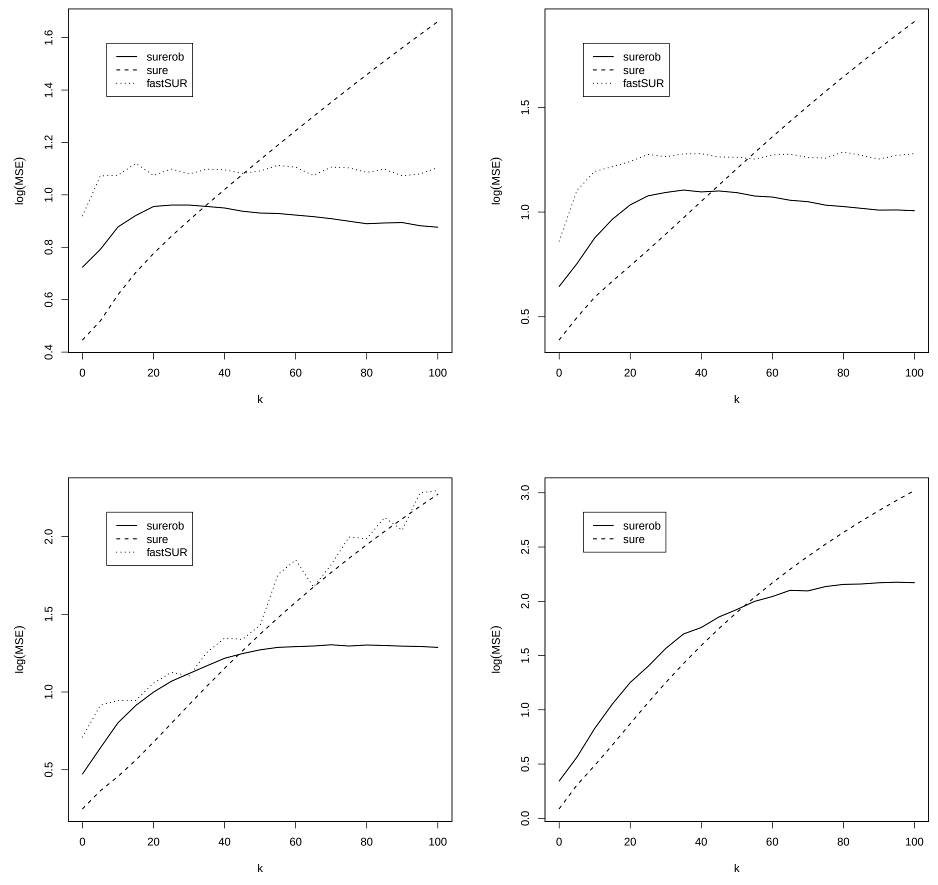


Figure 21: Mean Square Error MSE = MSE($\hat{\boldsymbol{\beta}}, \boldsymbol{\beta}$) for surerob (solid line), sure (dashed line) and FastSUR (dotted line) for different levels of contamination $\epsilon = 5\%$, $10\%$, (top) $20\%$, $30\%$ (bottom) under the THCM considering dimension $p = 10$ and number of equations $m = 20$.

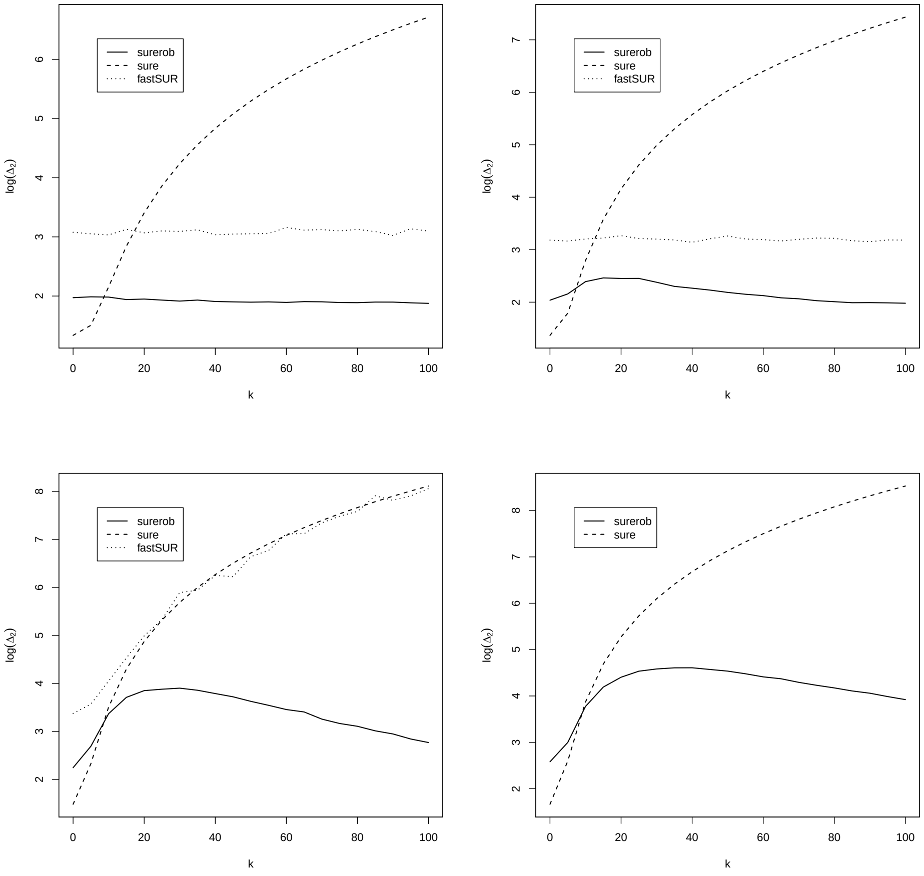


Figure 22: Average Kullback-Leibler $\Delta_2 = \Delta(\hat{\Sigma}_2, \Sigma)$ for surerob (solid line), sure (dashed line) and FastSUR (dotted line) for different levels of contamination $\epsilon = 5\%$, $10\%$, (top) $20\%$, $30\%$ (bottom) under the THCM considering dimension $p = 10$ and number of equations $m = 20$.

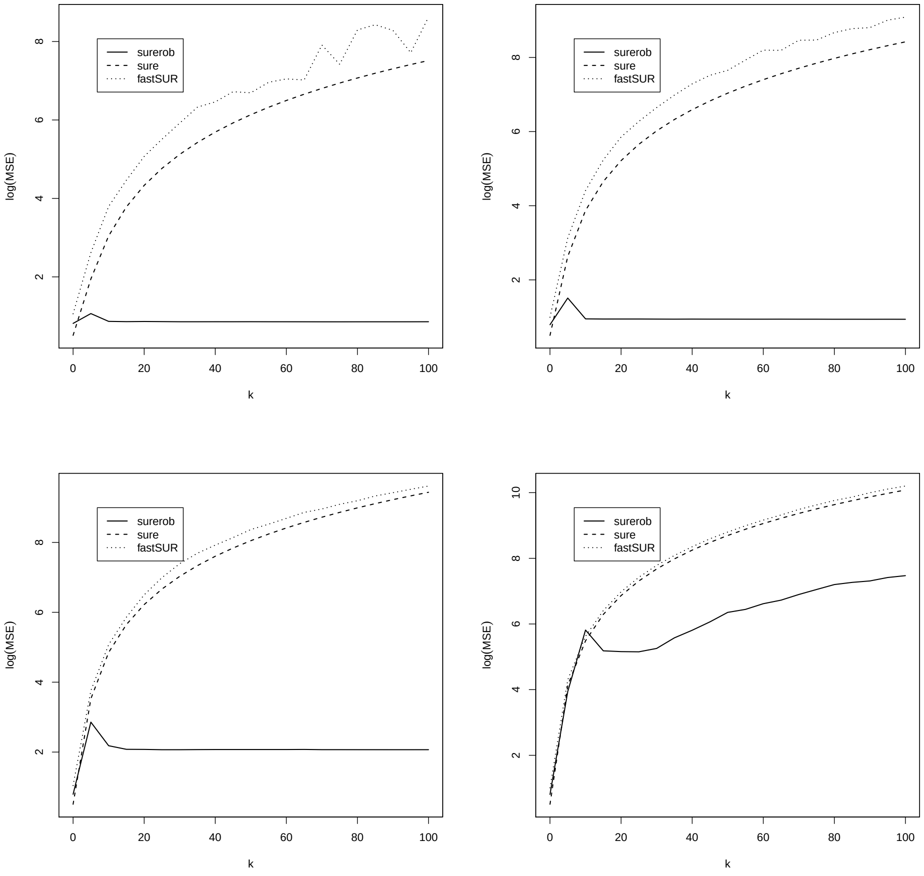


Figure 23: Mean Square Error MSE = MSE($\hat{\boldsymbol{\beta}}, \boldsymbol{\beta}$) for surerob (solid line), sure (dashed line) and FastSUR (dotted line) for different levels of contamination $\epsilon = 5\%$, $10\%$, (top) $20\%$, $30\%$ (bottom) under the ICM considering dimension $p = 10$ and number of equations $m = 20$.

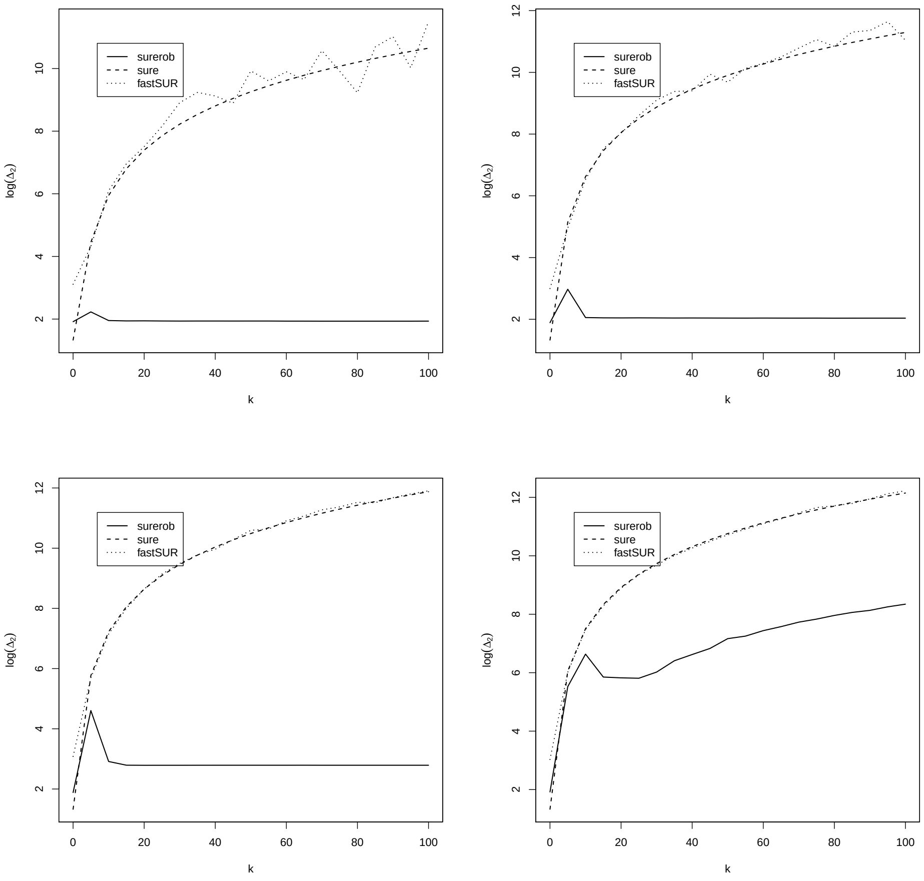


Figure 24: Average Kullback-Leibler $\Delta_2 = \Delta(\hat{\Sigma}_2, \Sigma)$ for surerob (solid line), sure (dashed line) and FastSUR (dotted line) for different levels of contamination $\epsilon = 5\%$, $10\%$, (top) $20\%$, $30\%$ (bottom) under the ICM considering $p = 10$ and number of equations $m = 20$.

# References

A. Henningsen and J.D. Hamann. systemfit: A package for estimating systems of simultaneous equations in R. *Journal of Statistical Software*, 23 (4):1–40, 2007. URL `http://www.jstatsoft.org/v23/i04/`.

J. Kmenta. *Elements of Econometrics*. Macmillan, New York, second edition edition, 1986.

A. Leung, M. Danilov, V.J. Yohai, and R.H. Zamar. *GSE: Robust Estimation in the Presence of Cellwise and Casewise Contamination and Missing Data*, 2019. URL `https://cran.r-project.org/web/packages/GSE`. R package version 4.2.

M. Mächler, P.J. Rousseeuw, C. Croux, V. Todorov, A. Ruckstuhl, M. Salibian-Barrera, T. Verbeke, M. Koller, E.L.T. Conceicao, and M. Anna di Palma. *robustbase: Basic Robust Statistics*, 2021. URL `http://robustbase.r-forge.r-project.org/`. R package version 0.93-8.
